# Supplementary material for: LatentDR: Improving Model Generalization Through Sample-Aware Latent Degradation and Restoration
Source: arXiv:2308.14596 source file (2023-08-28)
Supplement: Supplementary file 1 [file additional_backbone.tex]

\paragraph{Using another backbone.}
As discussed in \cite{cha2022domain}, when testing on domain generalization applications, it is not necessarily better to use larger-scale backbone models, as naively fine-tuning the pre-trained models on DG might worsen the performance. 
To validate the effectiveness of our method when using a larger-scale backbone, we selected ViT-B which is pre-trained on ImageNet-21k and benchmarked a few methods on top.
We show that our data augmentation operation is robust when testing with a larger-scale backbone, which demonstrates its potential when applied together with other models.

Performance on OfficeHome improves a lot for all the methods. But we are able to get a very strong performance as compared to others. A potential reason could be the difficulty of the OfficeHome dataset. PACS and VLCS have 7 and 5 classes each, but OfficeHome has 65 classes. And the three datasets have similar number of datapoints (9991, 10729, and 15588 respectively). Due to this, OfficeHome has a lot of room for improvement, hence a stronger backbone that is pre-trained on ImageNet-21k seems to utilize this potential and we are able to notice significant improvements in performance on this dataset.

\begin{table}[h!]
\caption{Results with a ViT backbone pre-trained on Imagenet.}
\vskip 0.15in
\begin{center}
%\begin{small}
% \begin{sc}
\begin{tabular}{lcccr}
\hline
& PACS & VLCS & OfficeHome & Avg. \\
\hline
CORAL & 85.9 & 75.3 & 75.3 & 78.8 \\
% MIRO &  &  &  & \\
ViT-B & 82.6 & 77.8 & 75.6 & 78.7 \\
+ Mixup & 84.8 & 76.9 & 75.7 & 79.1 \\
+ BF & 80.2 & 76.8 & 75.0 & 77.3 \\
\hline
+ Ours (SA) & 84.5 & 79.0 & 77.1 & 80.2 \\
+ Ours (Pool) & 86.4 & 78.6 & 77.3 & 80.8 \\
\hline
\end{tabular}
% \end{sc}
%\end{small}
\end{center}
\vskip -0.1in
\end{table}
