# Supplementary material for: LatentDR: Improving Model Generalization Through Sample-Aware Latent Degradation and Restoration
Source: arXiv:2308.14596 source file (2023-08-28)
Supplement: Supplementary file 2 [file additional_explain.tex]

\subsubsection{Intuitive explanation of latent degradation}

We provide more intuitive explanations of our latent degradation operation from the perspective of the Vicinal Risk Minimization (VRM) principle. 
% While the following contents aim to provide 
% , hoping to provide future research opportunities.
% \paragraph{Vicinal Risk Minimization (VRM).}
% below rewrote from Mixup
% below rewrote from Mixup
% below rewrote from Mixup
% need further edit (simplify)

The goal of supervised learning is to learn a function $f(\cdot)$ that studies the relationship between data $X$ and target $Y$, which follows the joint distribution $P(X, Y)$. Specifically, consider a loss function $\ell$, the goal is to minimize the expected risk:
\[
R(f)=\int \ell(f(x), y) \mathrm{d} P(x, y)
\]
where the goal is to minimize the expected loss over the data distribution $P$.

Unfortunately, the distribution $P$, in practice, is limited by the diversity of the training data. $(\mathcal{X}, \mathcal{Y})=\left\{\left(x_i, y_i\right)\right\}_{i=1}^n$, where $\left(x_i, y_i\right) \sim P$ for all $i$. The empirical distribution $P$ by the empirical distribution is approximated using the training data:
\[
P(x, y)=\frac{1}{n} \sum_{i=1}^n \delta\left(x=x_i, y=y_i\right),
\]
where $\delta\left(x=x_i, y=y_i\right)$ is a Dirac mass centered at $\left(x_i, y_i\right)$. 

What Mixup did is that:
\begin{gather*}
    %\begin{array}{r}
    \tilde{x}=\lambda x_i+(1-\lambda) x_j \\
    \tilde{y}=\lambda y_i+(1-\lambda) y_j \\
    %\end{array} \\
    \mu\left(\tilde{x}, \tilde{y} \mid x_i, y_i\right)=\frac{1}{n} \sum_j^n \underset{\lambda}{\mathbb{E}}\left[\delta\left(\tilde{x}, \tilde{y}\right)\right]
\end{gather*}
which replaces the original distribution such that:
\[
P_\nu(\tilde{x}, \tilde{y})=\frac{1}{n} \sum_{i=1}^n \nu\left(\tilde{x}, \tilde{y} \mid x_i, y_i\right)
\]
However, in reality, Mixup often selects $\alpha$ from a Beta distribution, which is often close to its original point, and provide limited diversity.

From this perspective, our degraded operator can be viewed as creating a non-convex version of Mixup.

% \paragraph{Content/style separation.}
% \paragraph{Preventing trivial solution.}

BatchFormer could obtain a trivial solution in the sense that the Transformer might just return an Identity matrix, although it has a high dropout rate. Our joint latent augmentation and label augmentation, instead, would prevent the trivial solution. Thus, it works even better, when combined with the restoration operator.
